# Supplementary material for: Fuzzing: On Benchmarking Outcome as a Function of Benchmark Properties
Source: arXiv:2212.09519 source file (2025-04-14)
Supplement: Supplementary file 1 [file supplementary.tex]

\section{Supplementary Analysis}
\todo{Use \autoref{fig:supCorrelation} to explain how we can improve the quality of the proportional odds logistic regression by excluding correlated co-variates.}

\begin{figure}
    \centering
    \includegraphics[width=\columnwidth]{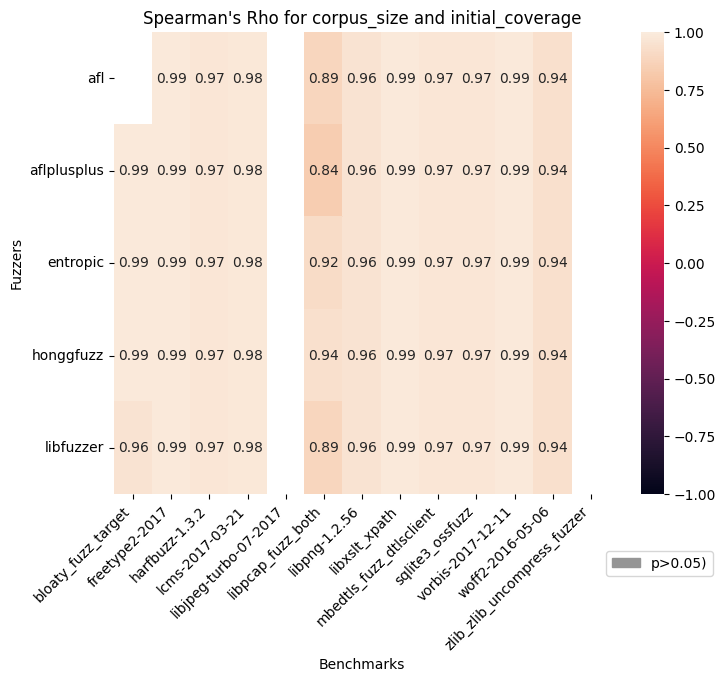}
    \caption{Since the size and initial coverage of the seed corpus are highly correlated, we should only use one of these properties for the proportional odds logistic regression. \todo{Too much unused whitespace. Increase "scale". Otherwise, use tabular and no colors.}}
    \label{fig:supCorrelation}
\end{figure}
